# Supplementary material for: Joint models for the longitudinal analysis of measurement scales in the presence of informative dropout
Source: arXiv:2110.02612 source file (2022-03-31)
Supplement: Supplementary file 1 [file suppmat_pdf.pdf]

# Supplementary material

# Joint models for the longitudinal analysis of measurement scales in the presence of informative dropout

Tiphaine Saulnier*, Viviane Philipps, Wassilios G Meissner, Olivier Rascol,
Anne Pavy-Le Traon, Alexandra Foubert-Samier, Cécile Proust-Lima

2022

## Simulation study with shared current level

This second simulation study illustrates the performances of the joint model in the case of current level dependency structure.

### Simulation design

We considered the setting of the time to a unique cause of event, and the repeated measures to 4 ordinal markers measuring the same underlying construct. The longitudinal part constitutes a dynamic Item Response Theory model for graded responses (see [23] in the same special issue). The longitudinal and survival processes were associated through the current latent process level (i.e., dependence structure defined in Equation (8)).

We simulated 500 samples of 300 subjects each. The structural model for the underlying process consisted in a linear function of time at the population ($\beta^L = (0, 1)^\top$) and individual level ($B = \left(\begin{smallmatrix} 1 & 0 \\ 0 & 0.2 \end{smallmatrix}\right)$). The time-to-event was defined by a Weibull baseline risk function $\lambda_0(t; \psi) = \psi_1^{\psi_2} \psi_2 t^{\psi_2 - 1}$ with $\psi_1 = 0.2, \psi_2 = 5$. The unique linear predictor was the current level of the underlying process with an association parameter fixed to $\alpha = 0.1$.

Visit times were generated every year (or time unit) from year 0 and up to the minimum between year 4 (administrative censoring) and the time-to-event. A delayed entry was generated to translate an individual-specific time of entry (year 0). To do so, we generated individual time-of-entry from a continuous uniform distribution defined on the interval [0,2]. This lead to a time-of-entry mean around 1.00 (SD=0.58), 26.07% of censoring on average and 3.45 repeated measures of each marker on average. The 4 markers had 4 ordinal levels each. The marker data were generated according to equation (5) with thresholds $\eta_1 = (0.5, 1, 1.5)^\top$, $\eta_2 = (0.25, 0.75, 0.8)^\top$, $\eta_3 = (0.1, 0.2, 0.4)^\top$ and $\eta_4 = (0.2, 0.4, 0.8)^\top$ and measurement error variances fixed to $\sigma = 1$.

### Results

We report in Table S1 the mean estimate, relative bias, variance estimate (empirical or asymptotic) and the coverage rate of the 95% confidence interval for each parameter. The estimation procedure provides very good results on this example: for all parameters, the bias is negligible, the mean asymptotic variance is close to the empirical variance, and the coverate rate of the 95% confidence interval is very close to the nominal value.

Table S 1: Summary on 500 replicates of the estimation of a joint model with 4 repeated ordinal markers and 1 event with latent process current level dependency structure on samples of 300 individuals.

| parameters | true value | mean estimate | relative bias (in %) | empirical standard deviation | mean asymptotic standard deviation | 95%CI coverage rate (in %) |
|---|---|---|---|---|---|---|
| ***survival model*** | | | | | | |
| baseline risk function (Weibull) | | | | | | |
| scale $\sqrt{\psi_1}$ | 0.447 | 0.448 | 0.1 | 0.008 | 0.008 | 93.6 |
| shape $\sqrt{\psi_2}$ | 2.236 | 2.252 | 0.7 | 0.069 | 0.070 | 95.2 |
| association parameter, $\alpha$ | 0.100 | 0.099 | -1.2 | 0.044 | 0.044 | 93.8 |
| ***structural model*** | | | | | | |
| adjustment covariates, $\beta^L$ | | | | | | |
| intercept | 1.000 | - | - | - | - | - |
| time | 1.000 | 1.023 | 2.3 | 0.137 | 0.131 | 93.8 |
| random effect covariance parameters, $B$ | | | | | | |
| choleski 0 | 1.000 | - | - | - | - | - |
| choleski 1 | 0.000 | 0.013 | - | 0.078 | 0.076 | 92.6 |
| choleski 2 | 0.447 | 0.445 | -0.6 | 0.073 | 0.068 | 90.6 |
| ***outcome-specific measurement model*** | | | | | | |
| thresholds for items | | | | | | |
| *item 1* | | | | | | |
| $\eta_{11}$ | 0.500 | 0.516 | 3.3 | 0.138 | 0.130 | 94.4 |
| $\eta_{12}$* | 0.707 | 0.712 | 0.7 | 0.053 | 0.052 | 94.6 |
| $\eta_{13}$* | 0.707 | 0.711 | 0.6 | 0.054 | 0.051 | 94.0 |
| *item 2* | | | | | | |
| $\eta_{21}$ | 0.250 | 0.262 | 4.8 | 0.126 | 0.124 | 95.0 |
| $\eta_{22}$* | 0.707 | 0.714 | 0.9 | 0.053 | 0.052 | 94.4 |
| $\eta_{23}$* | 0.224 | 0.220 | -1.5 | 0.041 | 0.041 | 94.0 |
| *item 3* | | | | | | |
| $\eta_{31}$ | 0.100 | 0.111 | 10.6 | 0.126 | 0.125 | 95.0 |
| $\eta_{32}$* | 0.316 | 0.320 | 1.1 | 0.047 | 0.046 | 94.2 |
| $\eta_{33}$* | 0.447 | 0.449 | 0.3 | 0.049 | 0.047 | 93.2 |
| *item 4* | | | | | | |
| $\eta_{41}$ | 0.200 | 0.206 | 3.0 | 0.126 | 0.123 | 93.6 |
| $\eta_{42}$* | 0.447 | 0.454 | 1.6 | 0.046 | 0.047 | 94.0 |
| $\eta_{43}$* | 0.632 | 0.638 | 0.8 | 0.051 | 0.050 | 95.0 |
| standard deviation from measurement error, $\sigma$ | | | | | | |
| item 1 | 1.000 | 1.017 | 1.7 | 0.132 | 0.126 | 93.8 |
| item 2 | 1.000 | 1.018 | 1.8 | 0.132 | 0.125 | 93.4 |
| item 3 | 1.000 | 1.016 | 1.6 | 0.136 | 0.128 | 93.0 |
| item 4 | 1.000 | 1.024 | 2.4 | 0.125 | 0.126 | 95.0 |

* squared root of the increment

## Additional figures and tables for the MSA application

Figure S 1: Survival submodel fit assessment through a graphical comparison between the observed survival curve and the predicted survival curves on 500 samples simulated from the fitted joint model.

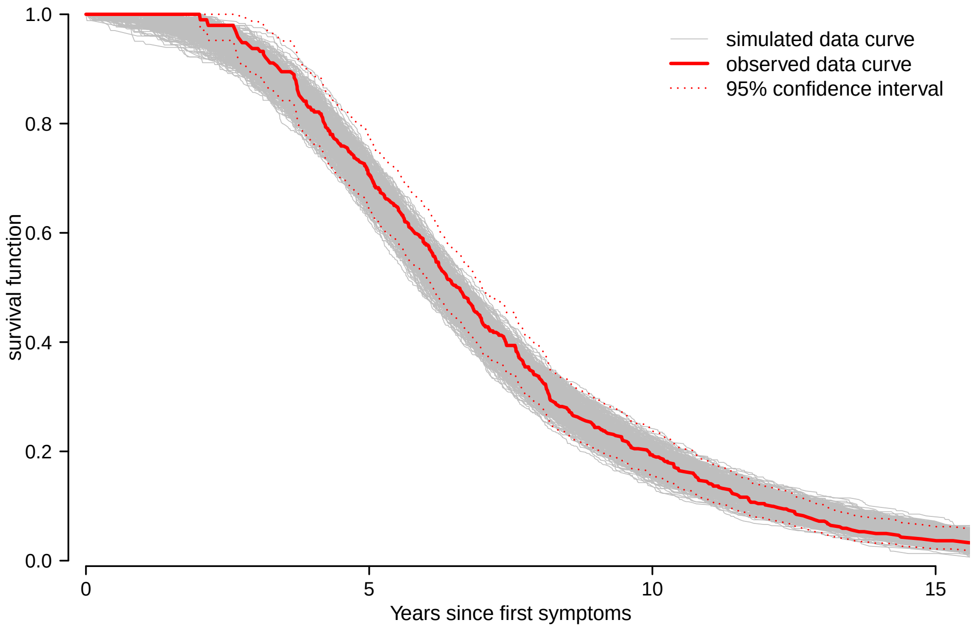


Figure S 2: Longitudinal submodel fit assessment through a graphical comparison between the observed item means and the predicted item means over discretized time.

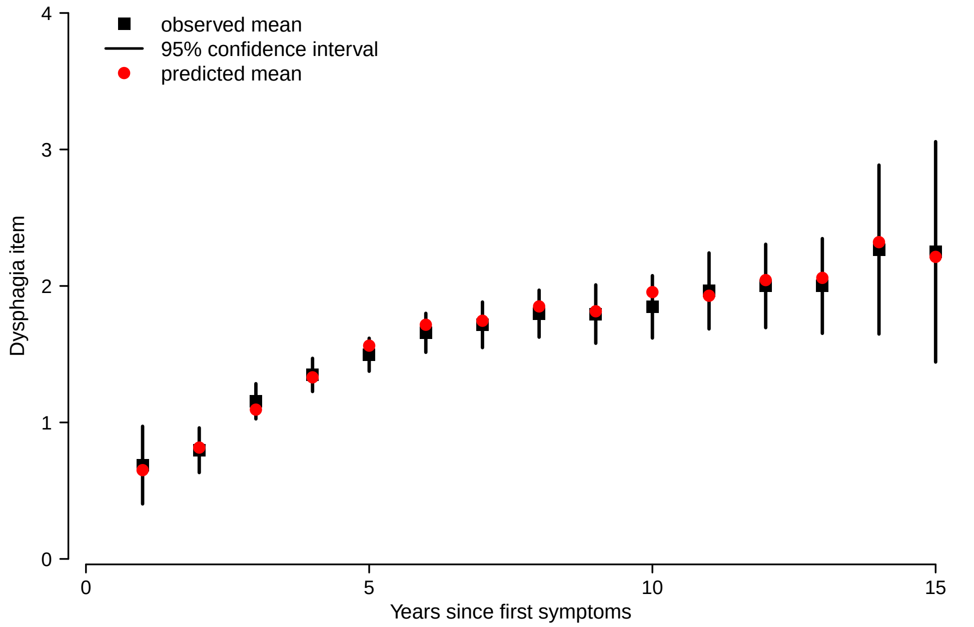


## Estimates of the shared random effect joint model in MSA application

Table S 2: Estimates of the shared random effect joint model in the MSA application to describe dysphagia progression (5-level ordinal item) and its strength association with death (more details about the model specification can be found in section 4.2).

| parameters | estimate | standard error | p-value |
|---|---|---|---|
| ***survival model*** | | | |
| baseline risk function, $\psi$ | | | |
| splines 1 | 0.000 | 0.053 | 1.00 |
| splines 2 | -0.090 | 0.149 | 0.54 |
| splines 3 | 0.262 | 0.062 | **<0.001** |
| splines 4 | 0.464 | 0.097 | **<0.001** |
| splines 5 | -0.385 | 0.133 | **<0.001** |
| splines 6 | 0.261 | 0.363 | 0.47 |
| splines 7 | 0.389 | 0.337 | 0.25 |
| linear predictors, $\beta^S$ | | | |
| sex, female | -0.190 | 0.115 | 0.10 |
| age | 0.269 | 0.072 | **0.04** |
| diagnosis, MSA-P | 0.124 | 0.123 | 0.31 |
| certainty, probable | 0.319 | 0.150 | **0.03** |
| association $\alpha$ | 1.328 | 0.192 | **<0.001** |
| ***structural model*** | | | |
| adjustment covariates, $\beta^L$ | | | |
| intercept | 0 | - | - |
| time | 0.214 | 0.062 | **<0.001** |
| time$^2$ | -0.005 | 0.004 | 0.19 |
| sex, female | -0.076 | 0.152 | 0.62 |
| age | 0.073 | 0.111 | 0.51 |
| diagnosis, MSA-P | 0.199 | 0.157 | 0.20 |
| certainty, probable | -0.421 | 0.216 | **0.05** |
| time : sex, female | 0.021 | 0.045 | 0.64 |
| time : age | 0.031 | 0.033 | 0.35 |
| time : diagnosis, MSA-P | -0.034 | 0.046 | 0.47 |
| time : certainty, probable | 0.155 | 0.064 | **0.01** |
| time$^2$ : sex, female | 0.000 | 0.003 | 0.97 |
| time$^2$ : age | -0.002 | 0.002 | 0.23 |
| time$^2$ : diagnosis, MSA-P | 0.000 | 0.003 | 0.97 |
| time$^2$ : certainty, probable | -0.006 | 0.004 | 0.11 |
| random effect covariance parameters, $B$ | | | |
| choleski 0 | 1 | - | - |
| choleski 1 | -0.242 | 0.018 | **<0.001** |
| choleski 2 | 0.091 | 0.020 | **<0.001** |
| choleski 3 | 0.009 | 0.001 | **<0.001** |
| choleski 4 | -0.004 | 0.002 | **<0.001** |
| choleski 5 | 0.000 | 0.001 | 0.15 |
| ***outcome-specific measurement model*** | | | |
| thresholds for the item | | | |
| $\eta_1$ | 0.402 | 0.215 | 0.06 |
| $\eta_2$* | 0.788 | 0.040 | **<0.001** |
| $\eta_3$* | 0.761 | 0.040 | **<0.001** |
| $\eta_4$* | 0.872 | 0.051 | **<0.001** |
| standard deviation from measurement error | | | |
| $\sigma$ | 0.343 | 0.038 | **<0.001** |

* squared root of the increment
